# Supplementary material for: Explaining a black-box using Deep Variational Information Bottleneck Approach
Source: arXiv:1902.06918 source file (2019-10-03)
Supplement: Supplementary file 4 [file eval_mi.tex]

\section{Fidelity}\label{eval-fidel}~\\
\begin{table}[h]
\centering

\begin{adjustbox}{max width=\textwidth}
\begin{threeparttable}
\caption{Mutual information on LSTM movie sentiment prediction model using IMDB.}
\label{eval-imdb-fidel-rationale}
\begin{tabular}{@{}cccccccccc@{}}
\toprule
 &  &  & L2X & \multicolumn{6}{c}{VIBI (Ours)} \\ \cmidrule(lr){4-4}\cmidrule(lr){5-10}
 & chunk size & k & 0 & 0.001 & 0.01 & 0.1 & 1 & 10 & 100 \\ \midrule
\multirow{4}{*}{IMDB} & sentence & 1 & 0.727 & 0.693 & 0.711 & 0.731 & 0.729 & \textbf{0.734} & \textbf{0.734} \\
 & word & 5 & 0.638 & 0.657 & \textbf{0.666} & 0.657 & 0.648 & 0.640 & 0.654 \\
 & 5 words & 1 & 0.601 & 0.630 & 0.624 & \textbf{0.632} & 0.628 & 0.623 & 0.628 \\
 & 5 words & 3 & \textbf{0.694} & 0.660 & 0.662 & 0.660 & 0.662 & 0.660 & 0.660 \\ \midrule
\multirow{4}{*}{MNIST} & sentence & 1 & 0.581 & 0.547 & 0.562 & 0.567 & 0.585 & \textbf{0.586} & \textbf{0.586} \\
 & word & 5 & 0.486 & 0.521 & \textbf{0.551} & 0.512 & 0.516 & 0.508 & 0.526 \\
 & 5 words & 1 & 0.478 & 0.506 & 0.500 & \textbf{0.540} & 0.501 & 0.498 & 0.504 \\
 & 5 words & 3 & \textbf{0.551} & 0.528 & 0.529 & 0.522 & 0.529 & 0.528 & 0.525 \\ \bottomrule
\end{tabular}
    \begin{tablenotes}
        \footnotesize
        \item Mutual information
    \end{tablenotes}
\end{threeparttable}
\end{adjustbox}
\end{table}
